# Supplementary material for: Identifying tax evasion in Mexico with tools from network science and machine learning
Source: arXiv:2104.13353 source file (2021-04-24)
Supplement: Supplementary file 1 [file appendix.tex]

\section*{Appendix}
\addcontentsline{toc}{section}{Appendix}

When placed at the end of a chapter or contribution (as opposed to at the end of the book), the
numbering of tables, figures, and equations in the appendix section continues on from that in the
main text. Hence please \textit{do not} use the \verb|appendix| command when writing an appendix at
the end of your chapter or contribution. If there is only one the appendix is designated
``Appendix'', or ``Appendix 1'', or ``Appendix 2'', etc. if there is more than one.

\begin{equation}
a \times b = c
\end{equation}
